# Supplementary material for: Interactive Multiscale Modeling to Bridge Atomic Properties and Electrochemical Performance in Li-CO$_2$ Battery Design
Source: arXiv:2501.10954 source file (2025-09-01)
Supplement: Supplementary file 1 [file SI.pdf]

# Supporting Information

## Interactive Multiscale Modeling to Bridge Atomic Properties and Electrochemical Performance in Li-$CO_2$ Battery Design

*Mohammed Lemaalem* [a,b], *Selva Chandrasekaran Selvaraj* [a,b], *Ilias Papailias* [c], *Naveen K. Dandu* [a,b], *Arash Namaeighasemi* [a], *Larry A. Curtiss* [b], *Amin Salehi-Khojin* [c], *and Anh T. Ngo* [a,b,*]

[a] Department of Chemical Engineering, University of Illinois Chicago, Chicago, IL60608, USA

[b] Materials Science Division, Argonne National Laboratory, Lemont, IL 60439, USA.

[c] Department of Mechanical Engineering, Lyle School of Engineering, SMU, 3101 Dyer Street.

*Corresponding author: anhngo@uic.edu, ango@anl.gov

CONTENTS

1. **Background:** Catalyst/electrolyte developments for Li-$CO_2$ battery.

2. **Supplementary notes:** Experimental setup.

3. **Supplementary notes:** Simulation detail.

4. **Figure S1.** Voltage-capacity curve during Li-$CO_2$ battery discharge at various rates ranging from 0.2 mA/cm$^2$ to 0.9 mA/cm$^2$.

5. **Figure S2.** Effect of initial values of relevant variables on the voltage-capacity curve during Li-$CO_2$ battery discharge at a rate of 0.4 mA/cm$^2$.

6. **Figure S3.** The change in porosity and volume fraction of the deposited species in the cathode throughout the discharge process at different current densities and discharge states.

7. **Figure S4.** The $CO_2$ concentration change in the cathode throughout the discharge process at different current densities and discharge states.

# 1 Background: Catalyst/electrolyte developments for Li-$CO_2$ battery.

The Li-$CO_2$ battery chemistry faces critical challenges in catalyst performance, primarily characterized by two fundamental issues, catalyst inefficiency and redox mediator limitations. Noble and transition metal catalysts (such as Pt and Au nanoparticles) demonstrate low catalytic activities for $CO_2$ reduction/evolution reactions in aprotic media, while 2D materials (e.g., $MoS_2$) exhibit poor structural stability at high current rates [26]. Existing catalysts struggle to maintain consistent performance across multiple charge-discharge cycles, often due to catalyst deactivation caused by self-degradation or environmental factors such as discharge product accumulation and species contamination [26]. Unlike Li-$O_2$

batteries, Li-$CO_2$ battery liquid catalysts are typically inactive in decomposing discharge products ($Li_2CO_3$ and solid carbon), and current redox mediators fail to effectively facilitate the reversible transformation of reaction intermediates [5]. The formation of $Li_2CO_3$, a wide-bandgap insulator, leads to slow kinetics and high voltage platforms ($> 4.3$ V) during the charging process, significantly decreasing the round-trip efficiency of the battery [14]. The lack of efficient decomposition mechanisms significantly impedes battery cycling efficiency, with most current Li-$CO_2$ batteries only capable of operating for dozens of cycles with low overpotential, even with state-of-the-art catalysts [26]. These challenges necessitate developing novel catalytic systems that can maintain high catalytic activity across extended cycling, demonstrate structural stability at elevated current rates, enable efficient decomposition of discharge products, and provide reversible electrochemical reactions with minimal energy loss. The development of catalysts with high catalytic activity and conductivity is crucial to the research of high-performance Li-$CO_2$ batteries [12]. Promising research directions in Li-$CO_2$ battery technology encompass a range of innovative approaches aimed at overcoming current limitations and enhancing overall performance [23, 14, 19]. Advanced solid redox mediators have shown significant potential, as demonstrated by a study using a Cu(II) coordination compound of benzene-1,3,5-tricarboxylic acid. This solid redox mediator enabled a Li-$CO_2$ battery to achieve a higher discharge voltage of 2.8 V, a lower charge potential of 3.7 V, and superior cycling performance over 400 cycles [23]. The use of solid redox mediators addresses the shuttle effect and sluggish kinetics associated with soluble redox mediators, potentially improving long-term stability and efficiency. Alternative reaction pathway engineering has emerged as another promising direction, focusing on promoting the formation of $Li_2C_2O_4$ instead of $Li_2CO_3$ as the discharge product. This approach can reduce the charge potential and improve overall battery performance [14]. For instance, the use of $Mo_2C$ as a cathode material has been shown to stabilize $Li_2C_2O_4$ as the final discharge product, reducing the charge potential to 3.8 V and enhancing the reversibility of the battery [14]. Innovative catalyst designs, including carbon-based and metal-complex catalysts, are being extensively

explored. Carbon-based materials, such as multi-walled carbon nanotubes (MWCNTs), are widely used as cathodes due to their high electrical conductivity and large surface area [19]. However, their limited catalytic activity for $Li_2CO_3$ decomposition has led to investigations of ways to enhance their performance, such as introducing metal catalysts like Ru to reduce overpotentials and improve efficiency [19]. Transition metal compound catalysts have shown promise in improving the catalytic activity and stability of Li-$CO_2$ batteries. For example, the integration of Ru-catalyzed MWCNT cathodes with solid electrolytes has demonstrated enhanced electrochemical reactions involving $CO_2$ [19]. Additionally, nanostructured catalyst development with improved conductivity and catalytic properties continues to be a focus area, exploring various materials and structures to optimize battery performance [9, 25, 18].

Ionic liquid-based electrolytes show promise for Li-$CO_2$ batteries due to their stability with intermediate products compared to solid-state electrolytes, but their development is limited by low ionic conductivity and high viscosity [26]. To address these limitations, ionic liquid electrolytes based on DMSO (dimethyl sulfoxide) as a solvent and LiTFSI (lithium bis(trifluoromethanesulfonyl)imide) as a salt, often incorporating EMIM-$BF_4$ (1-Ethyl-3-methylimidazolium tetrafluoroborate), have been developed [15, 27, 21, 24, 1, 10, 9]. These electrolytes are preferred for Li-$CO_2$ batteries due to their superior ionic conductivity, enhanced electrochemical stability, and improved $CO_2$ activation properties. DMSO-based electrolytes exhibit faster $Li^+$ ion diffusion kinetics compared to other solvents like TEGDME (tetraethylene glycol dimethyl ether), resulting in lower polarization potential [15]. Li-$CO_2$ batteries using 3M LiTFSI in DMSO electrolyte have demonstrated excellent cycling performance, maintaining stable operation for over 1,900 hours (180 cycles) [15]. In concentrated DMSO-based electrolytes, $TFSI^-$ anions can access the primary solvation sheath of $Li^+$ ions, leading to the formation of a LiF-rich solid electrolyte interphase (SEI) layer, which is beneficial for battery performance [27, 21]. DMSO-based electrolytes demonstrate good electrochemical stability with both the Li metal anode and the reactive cathode at high volt-

ages and elevated temperatures [15]. The use of DMSO-based electrolytes improves the rate capability of the battery, with cells able to deliver flat charge/discharge plateaus at current densities of up to 2,000 mA $g^{-1}$ [27]. Together, these properties make the DMSO LiTFSI electrolyte a promising choice for improving the overall performance and stability of Li-$CO_2$ batteries. The addition of EMIM-$BF_4$ (1-Ethyl-3-methylimidazolium tetrafluoroborate) as an electrolyte material plays several important roles in Li-$CO_2$ batteries. EMIM-$BF_4$ helps in activating $CO_2$ molecules, which is crucial for the $CO_2$ reduction reaction in Li-$CO_2$ batteries [24]. The addition of EMIM-$BF_4$ to the electrolyte has been shown to enhance battery performance. In one study, a Li-$CO_2$ battery using 0.1 M LiTFSI in (EMIM-$BF_4$)/DMSO as the electrolyte achieved 500 cycles at 0.5 A/g with a capacity of 500 mAh/g [15]. The presence of EMIM-$BF_4$ in the electrolyte contributes to improved cycling stability of Li-$CO_2$ batteries [1]. When combined with other electrolyte components like DMSO and LiTFSI, EMIM-$BF_4$ contributes to the overall performance enhancement of Li-$CO_2$ batteries, including higher discharge voltages and increased capacities [10]. Recently, Jaradat et al. used an electrolyte combination of $ZnI_2$, LiTFSI, DMSO, and EMIM-$BF_4$ with a volumetric ratio of 2:3 that led to good Li-$CO_2$ battery performance [9].

# 2 Supplementary notes: Experimental setup

## 2.1 Cathode preparation

To synthesize $Sb_{0.67}Bi_{1.33}Te_3$ nanoflakes (NFs), a powder sample weighing 100 mg was dispersed in 20 ml of isopropyl alcohol (IPA) and subjected to ultrasonication for a duration of 24 hours. Subsequently, the solution was centrifuged at 1000 RPM for 15 minutes, allowing for the extraction of the supernatant materials. The resulting $Sb_{0.67}Bi_{1.33}Te_3$ was then deposited onto carbon cloth with a mass loading of 0.4 mg and subsequently dried under ultraviolet (UV) light.

## 2.2 Electrolyte preparation

A mixture of 1M LiTFSI and 0.025M $ZnI_2$ was combined with a solution of DMSO and EMIM-BF4 ionic liquid in a ratio of 3:2. The preparation of the electrolyte was conducted within an argon-filled glove box, maintaining oxygen and humidity levels below 0.1 ppm to prevent contamination.

## 2.3 Battery assembly

The assembly of the battery was conducted within an argon-filled glove box, maintaining oxygen and humidity levels below 0.1 ppm. The process for assembling the 2032-type coin-cell battery was as follows: (i) the wave spring and spacer were inserted into the coin cell; (ii) a glass-fiber separator, along with 50 $\mu$l of electrolyte, was affixed to the anode; (iii) cathodes coated with $Sb_{0.67}Bi_{1.33}Te_3$ nanofibers were attached to the separator. Subsequently, holes were drilled, and the case assembly was secured to the top of the cathode. For the battery studies, a Galvanostatic Battery Analyzer (MTI Corp, BST8-MA) was employed. The cycling experiments were conducted within small, sealed bags filled with $CO_2$ at an ambient temperature of 25 °C.

## 2.4 Three electrodes set up

A three-electrode configuration was employed for conducting electrochemical Linear Sweep Voltammetry (LSV) experiments. The working electrode consisted of $Sb_{0.67}Bi_{1.33}Te_3$ nanofibers (NFs) coated cathodes, while lithium metal disks served as both the counter and reference electrodes. The electrolyte utilized for the electrochemical measurements was saturated with carbon dioxide ($CO_2$). The experiments were performed using a Voltalab potentiostat at a sweep rate of 5 mV/s.

# 3 Supplementary notes: Simulation detail

## 3.1 Detailed DFT Computational Parameters

DFT calculations employed the projector augmented wave (PAW) method to describe the valence electrons of Bi, Sb, Te, Li, C, and O atoms, using a plane-wave basis set with a kinetic energy cutoff of 500 eV [2]. The generalized gradient approximation of Perdew and Wang was used for exchange-correlation energy [20, 3]. The unit cells of both $Sb_{0.67}Bi_{1.33}Te_3$ and $Li_2CO_3$ were expanded to lattice constants greater than 20 Å to allow sampling of $1 \times 1 \times 1$ k-meshes. Structural optimization was performed by alternately minimizing ionic and electronic energies until all forces were less than ±10 meV/Å. For surface calculations, a k-mesh of $4 \times 4 \times 1$ was used, with a total energy convergence criterion of $1 \times 10^{-5}$ eV and force convergence below 0.001 eV/Å. The D3 van der Waals correction by Grimme was included in all calculations to accurately capture dispersion interactions, which are particularly important for modeling the physisorption of $CO_2$ on the catalyst surface.

## 3.2 Detailed MD Simulation Parameters

MD simulations employed a 14 Å cutoff for both Lennard-Jones and Coulomb interactions and a 1 fs time step. Long-range electrostatics were treated using the PPPM solver with an accuracy of $10^{-4}$ [17, 8]. Molecular geometries were optimized using the General Amber Force Field (GAFF) and Universal Force Field (UFF), and final GROMOS parameters for $TFSI^-$, DMSO, $EMIM^+$, $BF4^-$, and $CO_2$ were obtained from the Automated Topology Builder (ATB) [16, 22, 13]. The ATB parameter generation considers Lennard-Jones parameters refined against experimental solvation and pure liquid properties, parametrization and validation using a single-range 14 Å cutoff, atomic charges fitted to quantum mechanical electrostatic potentials, and bonded parameters assigned using force constants estimated at the B3LYP/6-31G* level of theory, resulting in robust symmetry routines for assigning identical parameters to chemically equivalent atoms, bonds, and angles. UFF was used for

$ZnI_2$, and $Li^+$ parameters were taken from the CL&P force field [4, 6]. Initial configurations were generated with Moltemplate [11] and energy minimized [7]. The system was agitated using the Langevin thermostat at 900 K for 1 ns, then with the Nosé-Hoover thermostat. Equilibration was performed in stages: cooling from 900 K to 300 K at 500 bar for 3 ns; reducing pressure from 500 bar to 1 bar at 300 K for 3 ns; and finally, equilibrating at 300 K and 1 bar for 10 ns.

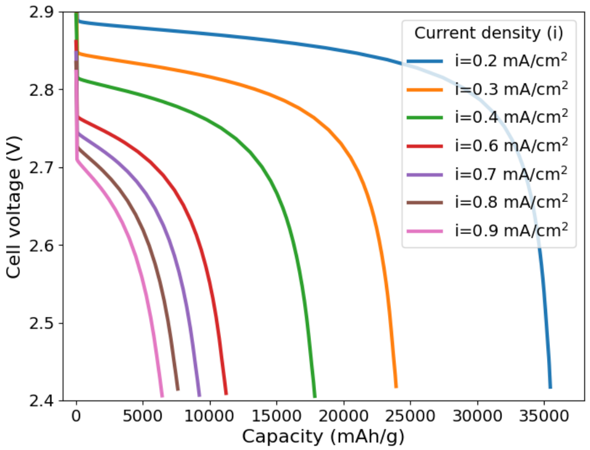


Figure S1: Voltage-capacity curve during Li-$CO_2$ battery discharge at various rates ranging from 0.2 mA/cm$^2$ to 0.9 mA/cm$^2$ supporting the data presented in Figure 3 (b), (c), and (d).

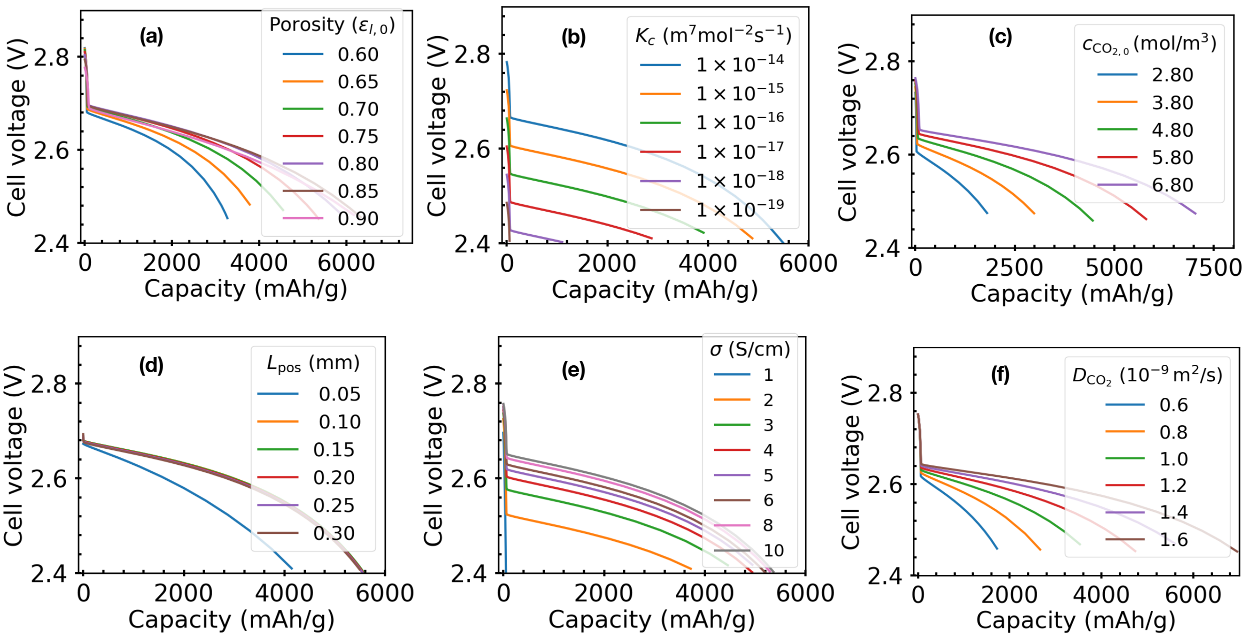


Impact of key parameters on voltage–capacity profiles: (a) Initial porosity ($\varepsilon_{l,0}$), (b) cathodic reaction rate constant ($K_c$), (c) initial $c_{CO_{2,0}}$ concentration, (d) cathode length ($L_{\text{pos}}$), (e) ionic conductivity ($\sigma$), and (f) CO2 diffusion coefficient ($D_{\text{CO}_2}$). The current density was held constant at 0.4 mA/cm$^2$; all other parameters are used as provided in Tables 1, 2, and 3. We note that the same qualitative behavior is observed for the other current densities considered in this work.

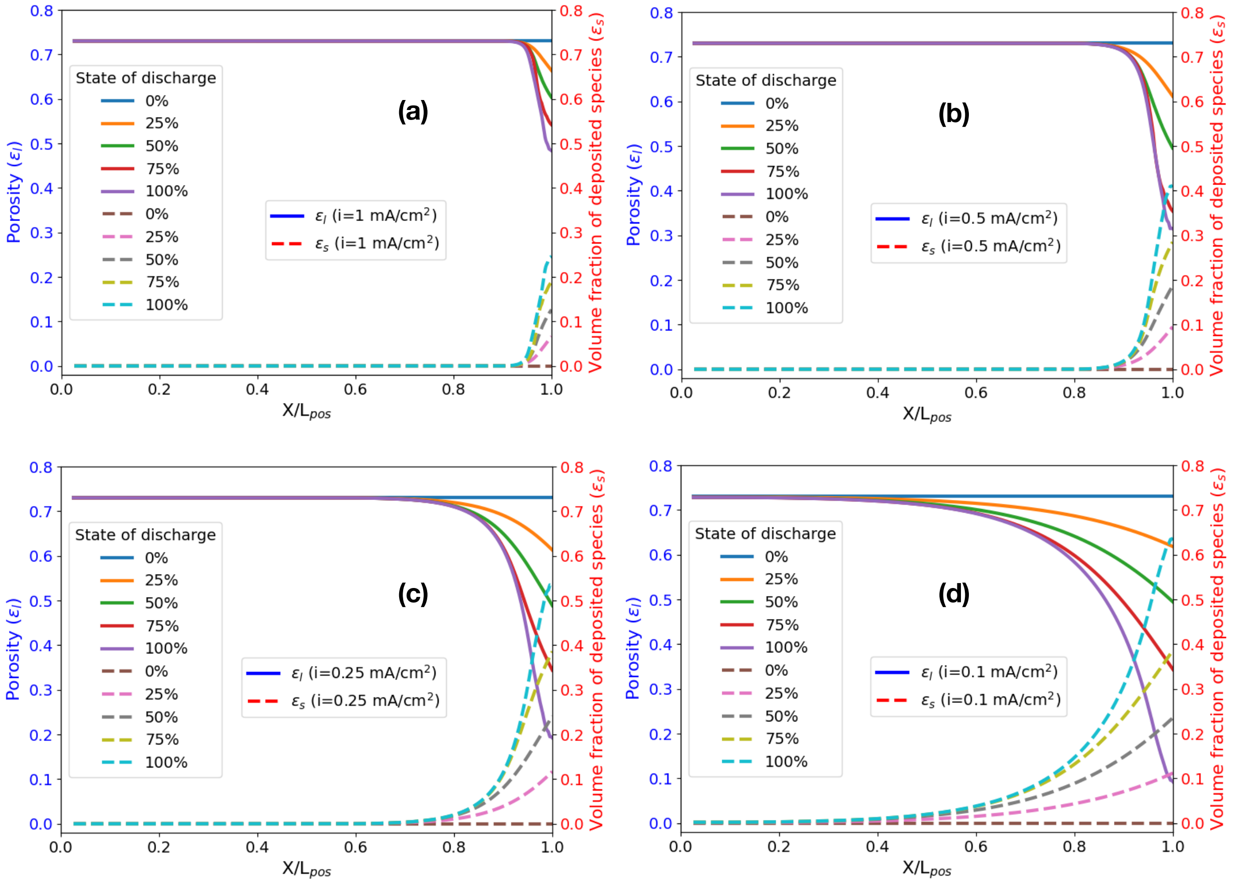


Figure S3: The change in porosity and volume fraction of deposited species in the cathode throughout the discharge process at different current densities ((a) 1, (b) 0.5, (c) 0.25, and (d) 0.1 mA/cm$^2$) in relation to the state of discharge. The distance (x) is normalized by the cathode length (L$_{pos}$).

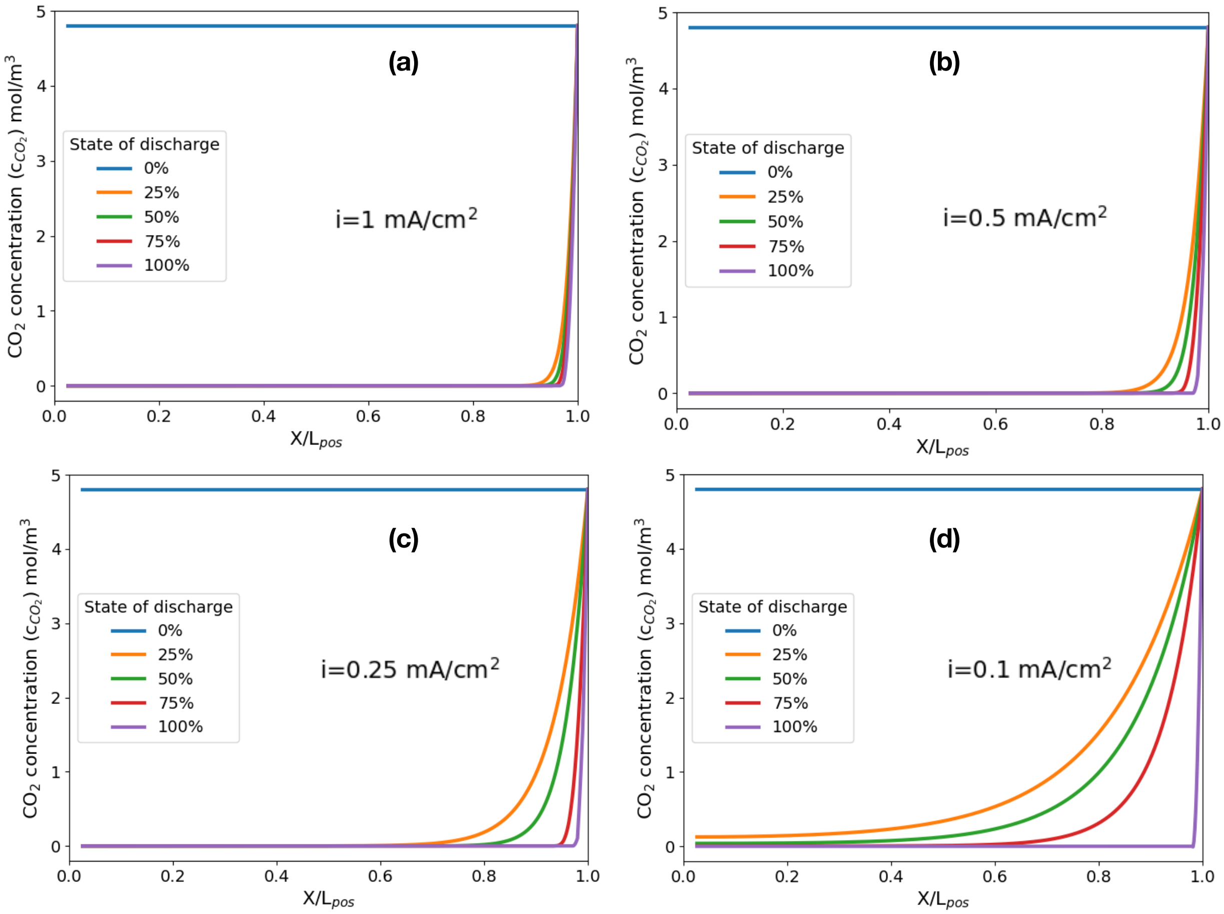


Figure S4: The local $CO_2$ concentration within the Li-$CO_2$ cathode during discharge was analyzed at various rates of 0.1, 0.25, 0.5, and 1 $mA/cm^2$, corresponding to different discharge levels (0 % indicates a fully charged battery). The distance (X) is normalized by the cathode length ($L_{pos}$).

# References


[1] Alireza Ahmadiparidari, Robert E Warburton, Leily Majidi, Mohammad Asadi, Amir Chamaani, Jacob R Jokisaari, Sina Rastegar, Zahra Hemmat, Baharak Sayahpour, Rajeev S Assary, et al. A long-cycle-life lithium-CO2 battery with carbon neutrality. *Advanced Materials*, 31(40):1902518, 2019.

[2] Peter E Blöchl. Projector augmented-wave method. *Physical review B*, 50(24):17953, 1994.

[3] Kieron Burke, John P Perdew, and Yue Wang. Derivation of a generalized gradient approximation: The PW91 density functional. In *Electronic Density Functional Theory: recent progress and new directions*, pages 81–111. Springer, 1998.

[4] José N Canongia Lopes and Agílio AH Pádua. CL&P: A generic and systematic force field for ionic liquids modeling. *Theoretical Chemistry Accounts*, 131(3):1–11, 2012.

[5] Yaying Dou, Zhaojun Xie, Yingjin Wei, Zhangquan Peng, and Zhen Zhou. Redox mediators for high-performance lithium-oxygen batteries. *National Science Review*, 9(4):nwac040, 2022.

[6] Kateryna Goloviznina, Zheng Gong, and Agilio AH Padua. The CL&Pol polarizable force field for the simulation of ionic liquids and eutectic solvents. *Wiley Interdisciplinary Reviews: Computational Molecular Science*, 12(3):e1572, 2022.

[7] Julien Guénolé, Wolfram G Nöhring, Aviral Vaid, Frédéric Houllé, Zhuocheng Xie, Aruna Prakash, and Erik Bitzek. Assessment and optimization of the fast inertial relaxation engine (fire) for energy minimization in atomistic simulations and its implementation in lammps. *Computational Materials Science*, 175:109584, 2020.

[8] Roger W Hockney and James W Eastwood. *Computer simulation using particles*. crc Press, 2021.

[9] Ahmad Jaradat, Musawenkosi K Ncube, Ilias Papailias, Nikhil Rai, Khagesh Kumar, Volodymyr Koverga, Roshan Y Nemade, Chengji Zhang, Nannan Shan, Hessam Shahbazi, et al. Fast charge-transfer rates in Li-CO2 batteries with a coupled cation-electron transfer process. *Advanced Energy Materials*, 14(15):2303467, 2024.

[10] Ahmad Jaradat, Chengji Zhang, Sanket Shashikant Sutar, Nannan Shan, Shuxi Wang, Sachin Kumar Singh, Taimin Yang, Khagesh Kumar, Kartikey Sharma, Shahriar Namvar, et al. A high-rate Li-CO2 battery enabled by 2D medium-entropy catalyst. *Advanced Functional Materials*, 33(21):2300814, 2023.

[11] Andrew I Jewett, David Stelter, Jason Lambert, Shyam M Saladi, Otello M Roscioni, Matteo Ricci, Ludovic Autin, Martina Maritan, Saeed M Bashusqeh, Tom Keyes, et al. Moltemplate: A tool for coarse-grained modeling of complex biological matter and soft condensed matter physics. *Journal of molecular biology*, 433(11):166841, 2021.

[12] Yanan Jiao, Jian Qin, Hirbod Maleki Kheimeh Sari, Dejun Li, Xifei Li, and Xueliang Sun. Recent progress and prospects of Li-CO2 batteries: Mechanisms, catalysts and electrolytes. *Energy Storage Materials*, 34:148–170, 2021.

[13] Katarzyna B Koziara, Martin Stroet, Alpeshkumar K Malde, and Alan E Mark. Testing and validation of the automated topology builder (ATB) version 2.0: prediction of hydration free enthalpies. *Journal of computer-aided molecular design*, 28(3):221–233, 2014.

[14] Wei Li, Menghang Zhang, Xinyi Sun, Chuanchao Sheng, Xiaowei Mu, Lei Wang, Ping He, and Haoshen Zhou. Boosting a practical Li-CO2 battery through dimerization reaction based on solid redox mediator. *Nature Communications*, 15(1):803, 2024.

[15] Zhenhua Lu, Min Xiao, Shuanjin Wang, Dongmei Han, Zhiheng Huang, Sheng Huang, and Yuezhong Meng. A rechargeable Li-CO2 battery based on the preservation of dimethyl sulfoxide. *Journal of Materials Chemistry A*, 10(26):13821–13828, 2022.

[16] Alpeshkumar K Malde, Le Zuo, Matthew Breeze, Martin Stroet, David Poger, Pramod C Nair, Chris Oostenbrink, and Alan E Mark. An automated force field topology builder (ATB) and repository: version 1.0. *Journal of chemical theory and computation*, 7(12):4026–4037, 2011.

[17] William McDoniel, Markus Höhnerbach, Rodrigo Canales, Ahmed E Ismail, and Paolo Bientinesi. LAMMPS'PPPM long-range solver for the second generation xeon phi. In *International Conference on High Performance Computing*, pages 61–78. Springer, 2017.

[18] Xiaowei Mu, Ping He, and Haoshen Zhou. Toward practical Li-CO2 batteries: Mechanisms, catalysts, and perspectives. *Accounts of Materials Research*, 2024.

[19] Dan Na, Dohyeon Yu, Hwan Kim, Baeksang Yoon, David D Lee, and Inseok Seo. Enhancing the performance and stability of Li-CO2 batteries through LAGTP solid electrolyte and MWCNT/Ru cathode integration. *Nanomaterials*, 14(23):1894, 2024.

[20] John P Perdew, Kieron Burke, and Matthias Ernzerhof. Generalized gradient approximation made simple. *Physical review letters*, 77(18):3865, 1996.

[21] Robert Pipes, Amruth Bhargav, and Arumugam Manthiram. Phenyl disulfide additive for solution-mediated carbon dioxide utilization in Li-CO2 batteries. *Advanced Energy Materials*, 9(21):1900453, 2019.

[22] Martin Stroet, Bertrand Caron, Koen M Visscher, Daan P Geerke, Alpeshkumar K Malde, and Alan E Mark. Automated topology builder version 3.0: Prediction of solvation free enthalpies in water and hexane. *Journal of chemical theory and computation*, 14(11):5834–5845, 2018.

[23] Juan Wang, Senlin Tian, Yang Lin, Haoran Song, Ningning Feng, Gang Yang, and Qun Zhao. Recent advancement in designing catalysts for rechargeable Li-CO2 batteries. *Catalysis Science & Technology*, 2024.

[24] Yunzhen Wu, Shuyan Cao, Jungang Hou, Zhuwei Li, Bo Zhang, Panlong Zhai, Yanting Zhang, and Licheng Sun. Rational design of nanocatalysts with nonmetal species modification for electrochemical CO2 reduction. *Advanced Energy Materials*, 10(29):2000588, 2020.

[25] Tengyu Yao, Zhenming Xu, Tingsong Hu, Kang Hu, Xueliang Cui, and Laifa Shen. High-throughput computation and machine learning prediction accelerating the design of cathode catalysts for Li-CO2 batteries. *The Journal of Physical Chemistry C*, 128(28):11534–11542, 2024.

[26] Shilin Zhang, Liang Sun, Qining Fan, Fangli Zhang, Zhijie Wang, Jinshuo Zou, Shiyong Zhao, Jianfeng Mao, and Zaiping Guo. Challenges and prospects of lithium-CO2 batteries. *Nano Research Energy*, 1(1), 2022.

[27] Wenchao Zhang, Fangli Zhang, Sailin Liu, Wei Kong Pang, Zhang Lin, Zaiping Guo, and Liyuan Chai. Regulating the reduction reaction pathways via manipulating the solvation shell and donor number of the solvent in Li-CO2 chemistry. *Proceedings of the National Academy of Sciences*, 120(14):e2219692120, 2023.
